# Supplementary material for: Safest Nearby Neighbor Queries in Road Networks (Full Version)
Source: arXiv:2107.14122 source file (2022-04-27)
Supplement: Supplementary file 1 [file 9_Appendix.tex]

\section{Proof of Lemma~\ref{ss_property2}}
\label{appendix1}
\begin{proof}
From Definition~\ref{def_PSS},  $pss(pt_{lj}) = \frac{1}{\sum_{s=1}^{s^{max}}{w_s \times pt_{lj}.d_s}}$. Replacing $pt_{lj}.d_s$ according to Definition~\ref{def_ds}, we have
%\begin{align*}
\begin{equation*}
  pss(pt_{lj}) = \frac{1}{\sum_{s=1}^{s^{max}}{w_s \times \sum_{e_{xy}\in pt_{lj} \wedge w_{xy}^{ss}=s} w^d_{xy}}}
 \end{equation*}
 
 \begin{equation*}
   = \frac{1}{\sum_{s=1}^{s^{max}}{w_s \times (\sum_{e_{xy}\in pt_{li} \wedge w_{xy}^{ss}=s} w^d_{xy} + \sum_{e_{xy}\in pt_{ij} \wedge w_{xy}^{ss}=s} w^d_{xy}})} 
\end{equation*}
\begin{equation*}
  =\frac{1}{\sum_{s=1}^{s^{max}}{(w_s \times \sum_{e_{xy}\in pt_{li} \wedge w_{xy}^{ss}=s} w^d_{xy}})+(w_s \times \sum_{e_{xy}\in pt_{ij} \wedge w_{xy}^{ss}=s} w^d_{xy})} 
 \end{equation*}
 \begin{equation*}
  =\frac{1}{(\sum_{s=1}^{s^{max}}{w_s \times pt_{li}.d_s})+(\sum_{s=1}^{s^{max}}{w_s \times pt_{ij}.d_s})} 
 \end{equation*}
 \begin{equation*}
  = \frac{1}{\frac{1}{pss(pt_{li})} + \frac{1}{pss(pt_{ij})}}
\end{equation*}
\qed
\end{proof}

\section{Proof of Lemma~\ref{lemma:pruning}}
\label{appendix2}
\begin{proof}
It is straightforward to show that $pt^\prime_{lj}\oplus pt_{jk}$ is at least as short as $pt_{lj}\oplus pt_{jk}$ because $pt^\prime_{lj}$ is at least as short as $pt_{lj}$ and $pt_{jk}$ is same in both paths. According to Lemma~\ref{ss_property2}, the PSS of $pt^\prime_{lj}\oplus pt_{jk}$ is $\frac{1}{\frac{1}{pss(pt^\prime_{lj})} + \frac{1}{pss(pt_{ik})}}$ and the PSS of $pt_{lj}\oplus pt_{jk}$ is $\frac{1}{\frac{1}{pss(pt_{lj})} + \frac{1}{pss(pt_{ik})}}$. $\frac{1}{pss(pt_{ik})}$ part is same in the PSS of both paths. Since $pss(pt^\prime_{lj}) \geq pss(pt_{lj})$,  $\frac{1}{\frac{1}{pss(pt^\prime_{lj})} + \frac{1}{pss(pt_{ik})}} \geq \frac{1}{\frac{1}{pss(pt_{lj})} + \frac{1}{pss(pt_{ik})}}$. Thus, $pt^\prime_{lj}\oplus pt_{jk}$ is at least as safe as $pt_{lj}\oplus pt_{jk}$.
\qed
\end{proof}
